# Supplementary material for: Interaction of water with nitrogen-doped graphene
Source: arXiv:2202.07970 source file (2022-02-16)
Supplement: Supplementary file 1 [file SM.pdf]

# Supplemental Material: Interaction of water with nitrogen-doped graphene

Azim Fitri Zainul Abidin and Ikutaro Hamada*

*Department of Precision Engineering,*

*Graduate School of Engineering, Osaka University,*

*2-1 Yamadaoka, Suita, 565-0871, Japan*

(Dated: February 16, 2022)

* ihamada@prec.eng.osaka-u.ac.jp

## SI. CONVERGENCE STUDY

We first performed the convergence study with respect to the **k**-point mesh, smearing function, smearing width ($\sigma$), and kinetic energy cutoffs for the wave functions ($E_{\rm cut}^{\rm wf}$) and augmentation charge ($E_{\rm cut}^{\rm den}$) using the different water/graphene configurations contained in the WaC18 data set[1] as shown in Tables SI, SII, SIII, SIV, SV, and SVI. We used both the PBE and rev-vdW-DF2 functionals for the convergence study. Converged interaction energies are summarized in Table SVII along with those obtained using various vdW-DF variants and converged computational parameters.

## SII. WATER ADSORPTION ON PRISTINE GRAPHENE

We calculated the interaction energy as a function of distance between water molecule and pristine graphene for the 0-leg, 1-leg, 2-leg, and para water configurations using PBE and rev-vdW-DF2 (Fig. 1 in the main text, Fig. S1 and Fig. S2). Three difference adsorption sites, namely, bridge, hollow, and on-top sites were considered as in previous studies [2, 3]. The equilibrium distance and the interaction energy at the equilibrium are summarized in Table SVIII. Our PBE results agree well with those reported in the literature[2, 3]. We can see that the interaction energies obtained using rev-vdW-DF2 is larger than those using PBE. We found that the energy difference among the different sites is negligibly small (<10 meV) , while that among the different water configurations (orientations) is much more prominent ($\sim$ 10 meV). This is explained by the fact that the water adsorption is governed by the dispersion interaction, while the water orientation is determined by the dipole of the water molecule and induced charge polarization. In the 0-leg configuration, the electronegative O atom induces charge depletion in the vicinity of the adsorption site, while electropositive H atoms in the 1-leg and 2-leg configurations induce charge accumulation. In the para configuration, on the other hand, the lone-pair orbital of the water molecule interacts repulsively with graphene, and the charge rearrangement in graphene is not significant. This argument is further corroborated by the fact that the energy differences among different orientations obtained using PBE are similar to those obtained using rev-vdW-DF2.

We investigated the dependence of the interaction energy on the lattice constant of graphene. The lattice constants obtained using PBE and rev-vdW-DF2 functionals are

listed in Table SIX. The interaction energy curves are shown in Fig. S3 and the equilibrium interaction energy and distance are summarized in Table SX. We can see that the equilibrium interaction energies and distances are almost identical to those obtained using the lattice constant of graphene optmized using PBE.

We also performed full structural optimization of the most stable adsorption configurations. The structure are shown in Fig. S4 and the interaction energies are summarized in Table SXI. We can see that the changes are minor and the results confirm that our conclusion is unchanged when the structural optimization is taken into account.

## SIII. ROLE OF THE DISPERSION INTERACTION IN WATER ADSORPTION

To clarify the role of nonlocal correlation, i.e., dispersion interaction, we decompose the interaction energy into the contributions from the nonlolcal correlation ($E_{\mathrm{c}}^{\mathrm{nl}}$) and the rest ($\Delta E^{\mathrm{vdW0}}$) for the selected adsorption configuration (Fig. S5). In the case of the pristine graphene, $\Delta E^{\mathrm{vdW0}}$ is purely repulsive, indicating that the dispersion interaction is solely responsible for the adsorption. In the case of the N-doped graphene on the other hand, $\Delta E^{\mathrm{vdW0}}$ is slightly attractive. Given that there is no significant hybridization of molecular orbitals and graphene states, we concluded that the attractive interaction is mainly ascribed to the ionic interaction between water and N-doped graphene.

## SIV. WATER ADSORPTION ON GRAPHENE DOPED WITH GRAPHITIC N

We considered water adsorbed on graphene doped with graphitic-N in parallel (para) configurations (Fig. S6). Calculated interaction energy curves for different N positions are shown in Fig. S7 and the equilibrium interaction energies and distances are summarized in Table SXII. We found that water in the para configuration [para 2, Fig. S6 (b)] with N2 is the most stable, and the interaction energy is comparable with that for the most stable 0-leg configuration, because the graphitic-N is positively charged. We also considered water adsorption on the on-top site adsorption in the 0-leg configuration with different N-positions (Fig. S8). Equilibrium interaction energies and distances are summarized in Table. SXIII.

## SV. WATER ADSORPTION ON GRAPHENE DOPED WITH PYRIDINIC-N

We then considered water adsorbed on graphene structure doped with pyridinic-N and non-H-terminated C [pyri-N (no H)] that with pyridinic-N and H-terminated C [pyri-N] in different orientations (Figs. S9 and S10). For 1-leg and 2-leg configurations, two water orientations were taken into account (1-leg 1, 1-leg 2, 2-leg 1, and 2-leg 2). Interaction energy curves of water in 0-leg, 1-leg 1, and 2-leg 1 configurations for graphene with pyri-N (no H) are shown in Fig. S11, and those in 0-leg, 1-leg 2, 2-leg 2, and para configurations are shown in Fig. S12. Equilibrium interaction energies and distances are summarized in Table SXIV (those for 1-leg 1 and 2-leg 1 configurations are shown in the main text). Generally, the interaction energy for those with dangling C atoms (no-H-terminated C atoms) is much larger than that with H-terminated C atoms, because the former is more reactive and H atoms interact repulsively with the water molecule.

We also calculated the interaction energies as functions of rotation angle for the 1-leg and para configurations on graphene with pyri-N, to investigate the angle of the water molecule precisely and to confirm that the water configurations employed in this work (0- 1-, and 2-leg configurations) are representative ones to describe water on N-doped graphene. For the 1-leg configuration, rotation angle of 0 degree gives the minimum, while $\sim$240 degree a local minimum, which correspond to the 1 leg in the configurations 1 and 2, respectively [Fig. S13(a)]. See also Fig. S10 for the water configurations. For the para configuration, rotation angle of $\sim$300 degree give the minimum, which corresponds approximately to the 2-leg configuration [Fig. S13(b)]. In the minimum configuration, the dipole of the water molecule does not direct precisely toward the surface as in the case of 2-leg configuration, because of the shorter distance and of the (larger) interaction with the terminating H atoms.

Furthermore, we performed full structural optimization of water in the 0- and 2-leg and para configurations. We found that water molecules in 0-leg and para configurations tilt by $\sim$31 and $\sim$55 degrees, respectively, and gain energies by 10 and 5 meV, respectively, and that the water in the 2-leg configuration is relaxed to the one similar to that similar to 1-leg configuration with the energy gain of 33 meV, because of the attractive interaction with pyri-N (Fig. S14).

## SVI. ELECTRONIC STRUCTURE ANALYSIS

We calculated the density of states (DOS) for pristine and N-doped graphene (Fig. S15) and the wave functions corresponding to the molecular orbitals (MOs) of water molecules in most stable adsorption configurations (Fig. S16). A $6 \times 6$ **k**-point mesh was used for the DOS calculations. We confirmed that the hybridization of water MOs with the graphene wave functions is negligibly small, and the character of the water MOs is retained upon adsorption.

Figures S17, S18, S19, and S20 show the calculated charge density differences ($\Delta\rho$) for different water configurations and N configurations. Overall, characteristics of $\Delta\rho$ are similar, when the water configurations are the same, and the degrees of the polarization differ depending on the N position.

Figure S21 shows the Hartree potential difference for the graphene doped with pyridinic-N and non-H-terminated C. This is very similar to the Hartree potential difference for the pyridinic-N case with H-terminated C atoms, except for the potential difference in the vicinity of the dangling C atoms.

Bader and Löwdin charges for graphene doped with graphitic-N and pyridinic-N are shown in Figs. S22 and S23, respectively. In the case of N-doped graphene, Bader and Löwdin charges are not always consistent, and the determination of the charge state of these systems based on the charge analysis needs great care.

TABLE SI. Interaction energies (in meV) for the 0-leg configuration obtained using difference computational parameters.

| **k**-point mesh | | Γ | | | 2 × 2 | | | 4 × 4 | | |
|---|---|---|---|---|---|---|---|---|---|---|
| $\sigma$ (Ry) | | 0.01 | 0.02 | 0.04 | 0.01 | 0.02 | 0.04 | 0.01 | 0.02 | 0.04 |
| $E_{cut}^{wf}$ | $E_{cut}^{den}$ | Methfessel-Paxton smearing | | | | | | | | |
| 80 | 640 | −9 | −9 | −9 | −8 | −10 | −9 | −8 | −9 | −9 |
| 80 | 800 | −10 | −10 | −9 | −9 | −10 | −9 | −8 | −9 | −9 |
| 80 | 960 | −10 | −10 | −10 | −9 | −9 | −9 | −8 | −9 | −9 |
| **k**-point mesh | | Γ | | | 2 × 2 | | | 4 × 4 | | |
| $\sigma$ (Ry) | | 0.01 | 0.02 | 0.04 | 0.01 | 0.02 | 0.04 | 0.01 | 0.02 | 0.04 |
| $E_{cut}^{wf}$ | $E_{cut}^{den}$ | Marzari-Vanderbilt smearing | | | | | | | | |
| 80 | 640 | −10 | −9 | −8 | −8 | −8 | −8 | −8 | −8 | −8 |
| 80 | 800 | −10 | −10 | −9 | −9 | −9 | −9 | −9 | −9 | −9 |
| 80 | 960 | −10 | −10 | −9 | −9 | −9 | −9 | −9 | −9 | −9 |

TABLE SII. Interaction energies (in meV) for the 1-leg configuration obtained using difference computational parameters.

| **k**-point mesh | | Γ | | | 2 × 2 | | | 4 × 4 | | |
|---|---|---|---|---|---|---|---|---|---|---|
| $\sigma$ (Ry) | | 0.01 | 0.02 | 0.04 | 0.01 | 0.02 | 0.04 | 0.01 | 0.02 | 0.04 |
| $E_{\text{cut}}^{\text{wf}}$ | $E_{\text{cut}}^{\text{den}}$ | Methfessel-Paxton smearing | | | | | | | | |
| 80 | 640 | −27 | −26 | −27 | −26 | −28 | −26 | −26 | −26 | −26 |
| 80 | 800 | −27 | −27 | −27 | −26 | −29 | −26 | −26 | −26 | −26 |
| 80 | 960 | −28 | −27 | −27 | −26 | −29 | −26 | −26 | −26 | −26 |
| **k**-point mesh | | Γ | | | 2 × 2 | | | 4 × 4 | | |
| $\sigma$ (Ry) | | 0.01 | 0.02 | 0.04 | 0.01 | 0.02 | 0.04 | 0.01 | 0.02 | 0.04 |
| $E_{\text{cut}}^{\text{wf}}$ | $E_{\text{cut}}^{\text{den}}$ | Marzari-Vanderbilt smearing | | | | | | | | |
| 80 | 640 | −27 | −27 | −26 | −26 | −27 | −26 | −26 | −26 | −26 |
| 80 | 800 | −28 | −27 | −26 | −26 | −26 | −26 | −26 | −26 | −26 |
| 80 | 960 | −28 | −27 | −27 | −26 | −26 | −26 | −26 | −26 | −26 |

TABLE SIII. Interaction energies (in meV) for the 2-leg configuration obtained using difference computational parameters.

| **k**-point mesh | | Γ | | | 2 × 2 | | | 4 × 4 | | |
|---|---|---|---|---|---|---|---|---|---|---|
| $\sigma$ (Ry) | | 0.01 | 0.02 | 0.04 | 0.01 | 0.02 | 0.04 | 0.01 | 0.02 | 0.04 |
| $E_{\text{cut}}^{\text{wf}}$ | $E_{\text{cut}}^{\text{den}}$ | Methfessel-Paxton smearing | | | | | | | | |
| 80 | 640 | −19 | −19 | −19 | −18 | −20 | −18 | −18 | −18 | −19 |
| 80 | 800 | −20 | −19 | −19 | −19 | −20 | −19 | −19 | −19 | −19 |
| 80 | 960 | −20 | −20 | −19 | −19 | −20 | −19 | −19 | −19 | −19 |
| **k**-point mesh | | Γ | | | 2 × 2 | | | 4 × 4 | | |
| $\sigma$ (Ry) | | 0.01 | 0.02 | 0.04 | 0.01 | 0.02 | 0.04 | 0.01 | 0.02 | 0.04 |
| $E_{\text{cut}}^{\text{wf}}$ | $E_{\text{cut}}^{\text{den}}$ | Marzari-Vanderbilt smearing | | | | | | | | |
| 80 | 640 | −19 | −19 | −18 | −18 | −19 | −18 | −18 | −18 | −19 |
| 80 | 800 | −20 | −20 | −19 | −19 | −19 | −19 | −19 | −19 | −19 |
| 80 | 960 | −20 | −20 | −19 | −19 | −19 | −19 | −19 | −19 | −19 |

TABLE SIV. Interaction energies (in meV) for the 0-leg configuration obtained using difference computational parameters, with rev-vdW-DF2 functional.

| **k**-point mesh | | Γ | | | 2 × 2 | | | 4 × 4 | | |
|---|---|---|---|---|---|---|---|---|---|---|
| σ (Ry) | | 0.01 | 0.02 | 0.04 | 0.01 | 0.02 | 0.04 | 0.01 | 0.02 | 0.04 |
| $E_{cut}^{wf}$ | $E_{cut}^{den}$ | Methfessel-Paxton smearing | | | | | | | | |
| 80 | 640 | −105 | −105 | −104 | −104 | −105 | −106 | −103 | −105 | −105 |
| 80 | 800 | −105 | −105 | −104 | −105 | −105 | −104 | −103 | −105 | −105 |
| 80 | 960 | −106 | −105 | −105 | −105 | −105 | −105 | −104 | −105 | −105 |
| **k**-point mesh | | Γ | | | 2 × 2 | | | 4 × 4 | | |
| σ (Ry) | | 0.01 | 0.02 | 0.04 | 0.01 | 0.02 | 0.04 | 0.01 | 0.02 | 0.04 |
| $E_{cut}^{wf}$ | $E_{cut}^{den}$ | Marzari-Vanderbilt smearing | | | | | | | | |
| 80 | 640 | −104 | −104 | −104 | −105 | −105 | −105 | −104 | −105 | −105 |
| 80 | 800 | −105 | −105 | −104 | −104 | −104 | −104 | −105 | −104 | −104 |
| 80 | 960 | −104 | −105 | −104 | −104 | −105 | −105 | −105 | −105 | −105 |

TABLE SV. Interaction energies (in meV) for the 1-leg configuration obtained using difference computational parameters, with rev-vdW-DF2 functional.

| **k**-point mesh | | Γ | | | 2 × 2 | | | 4 × 4 | | |
|---|---|---|---|---|---|---|---|---|---|---|
| σ (Ry) | | 0.01 | 0.02 | 0.04 | 0.01 | 0.02 | 0.04 | 0.01 | 0.02 | 0.04 |
| $E_{cut}^{wf}$ | $E_{cut}^{den}$ | Methfessel-Paxton smearing | | | | | | | | |
| 80 | 640 | −111 | −110 | −109 | −110 | −111 | −110 | −110 | −110 | −110 |
| 80 | 800 | −111 | −110 | −110 | −110 | −111 | −110 | −109 | −110 | −109 |
| 80 | 960 | −112 | −111 | −110 | −110 | −110 | −109 | −110 | −110 | −110 |
| **k**-point mesh | | Γ | | | 2 × 2 | | | 4 × 4 | | |
| σ (Ry) | | 0.01 | 0.02 | 0.04 | 0.01 | 0.02 | 0.04 | 0.01 | 0.02 | 0.04 |
| $E_{cut}^{wf}$ | $E_{cut}^{den}$ | Marzari-Vanderbilt smearing | | | | | | | | |
| 80 | 640 | −109 | −109 | −110 | −110 | −111 | −110 | −110 | −110 | −110 |
| 80 | 800 | −111 | −110 | −110 | −110 | −110 | −110 | −110 | −110 | −110 |
| 80 | 960 | −111 | −111 | −111 | −110 | −110 | −110 | −110 | −110 | −110 |

TABLE SVI. Interaction energies (in meV) for the 2-leg configuration obtained using difference computational parameters, with rev-vdW-DF2 functional.

| **k**-point mesh | | Γ | | | 2 × 2 | | | 4 × 4 | | |
|---|---|---|---|---|---|---|---|---|---|---|
| $\sigma$ (Ry) | | 0.01 | 0.02 | 0.04 | 0.01 | 0.02 | 0.04 | 0.01 | 0.02 | 0.04 |
| $E_{\mathrm{cut}}^{\mathrm{wf}}$ | $E_{\mathrm{cut}}^{\mathrm{den}}$ | Methfessel-Paxton smearing | | | | | | | | |
| 80 | 640 | −115 | −115 | −115 | −116 | −116 | −115 | −115 | −114 | −114 |
| 80 | 800 | −114 | −115 | −115 | −115 | −115 | −115 | −115 | −115 | −115 |
| 80 | 960 | −115 | −116 | −116 | −115 | −116 | −116 | −116 | −115 | −115 |
| **k**-point mesh | | Γ | | | 2 × 2 | | | 4 × 4 | | |
| $\sigma$ (Ry) | | 0.01 | 0.02 | 0.04 | 0.01 | 0.02 | 0.04 | 0.01 | 0.02 | 0.04 |
| $E_{\mathrm{cut}}^{\mathrm{wf}}$ | $E_{\mathrm{cut}}^{\mathrm{den}}$ | Marzari-Vanderbilt smearing | | | | | | | | |
| 80 | 640 | −115 | −115 | −116 | −114 | −115 | −115 | −115 | −117 | −115 |
| 80 | 800 | −116 | −116 | −115 | −115 | −115 | −115 | −115 | −115 | −115 |
| 80 | 960 | −113 | −115 | −114 | −115 | −115 | −115 | −115 | −115 | −115 |

TABLE SVII. Summary of the interaction energies (in meV) for water on graphene in 0-leg, 1-leg, and 2-leg configurations from the WAC18 dataset using various vdW-DF functionals, along with those using PBE and rev-vdW-DF2 reported by Brandenburg *et al.* [1] $E_{\mathrm{cut}}^{\mathrm{wf}}(E_{\mathrm{cut}}^{\mathrm{den}}) = 80(800)$ Ry, The Marzari-Vanderbilt smearing with $\sigma = 0.02$ Ry, and the Γ-point for the Brillouin zone sampling was used.

| | 0-leg | 1-leg | 2-leg |
|---|---|---|---|
| PBE[a] | −10 | −27 | −19 |
| rev-vdW-DF2[a] | −105 | −110 | −116 |
| vdW-DF2-C09[a] | −71 | −76 | −75 |
| vdW-DF-cx[a] | −130 | −134 | −133 |
| vdW-DF3-opt1[a] | −117 | −121 | −127 |
| vdW-DF3-opt2[a] | −119 | −123 | −130 |
| vdW-DF-cx0[a] | −146 | −142 | −‘48 |
| rev-vdW-DF2-0[a] | −111 | −108 | −115 |
| PBE[b] | −9 | −26 | −19 |
| rev-vdW-DF2[b] | −105 | −110 | −115 |
| DMC[b] | $-90 \pm 6$ | $-92 \pm 6$ | $-99 \pm 6$ |

[a] This work
[b] Ref. 1

TABLE SVIII. Equilibrium interaction energy ($E_{\mathrm{int}}$) and distance ($d_0$) of water on pristine graphene with difference configurations at different adsorption sites obtained using PBE and rev-vdW-DF2 functionals.

| Configuration | Adsorption site | PBE | | rev-vdW-DF2 | |
|---|---|---|---|---|---|
| | | $E_{\mathrm{int}}$ (meV) | $d_0$ (Å) | $E_{\mathrm{int}}$ (meV) | $d_0$ (Å) |
| 0-leg | Bridge | −20 | 3.549 | −98 | 3.123 |
| | Hollow | −22 | 3.513 | −106 | 3.049 |
| | On top | −20 | 3.549 | −99 | 3.102 |
| 1-leg | Bridge | −31 | 3.672 | −112 | 3.401 |
| | Hollow | −27 | 3.699 | −103 | 3.438 |
| | On top | −32 | 3.672 | −113 | 3.401 |
| 2-leg | Bridge | −25 | 3.624 | −111 | 3.363 |
| | Hollow | −27 | 3.608 | −116 | 3.321 |
| | On top | −24 | 3.635 | −107 | 3.389 |
| Para | Bridge | −18 | 4.153 | −96 | 3.773 |
| | Hollow | −19 | 4.122 | −102 | 3.735 |
| | On top | −18 | 4.153 | −95 | 3.773 |

TABLE SIX. Optimized lattice constant for pristine graphene obtained using PBE and rev-vdW-DF2 functionals.

| Functional | Lattice constant (Å) |
|---|---|
| PBE | 2.467 |
| rev-vdW-DF2 | 2.465 |

TABLE SX. Interaction energy at the equilibrium ($E_0$) and the equilibrium distance ($d_0$) of water on pristine graphene obtained using rev-vdW-DF2 and the lattice constant optimized using rev-vdW-DF2.

| Configuration | $E_0$ (meV) | $d_0$ (Å) |
|---|---|---|
| 0-leg | −106 | 3.055 |
| 1-leg | −114 | 3.411 |
| 2-leg | −116 | 3.334 |

TABLE SXI. Interaction energies ($E_{\mathrm{int}}$) for fully optimized most stable water adsorption configurations on pristine graphene, graphene doped with graphitic-N without H termination, and graphene doped with pyridinic-N with H termination obtained using rev-vdW-DF2.

| Configuration | $E_{\mathrm{int}}$ (meV) |
|---|---|
| 2-leg (graphene) | −132 |
| 0-leg (graphitic-N) | −156 |
| 1-leg (pyridinic-N) | −186 |

TABLE SXII. Equilibrium interaction energies ($E_{\mathrm{int}}$) and distance ($d_0$) of water on graphene doped with graphitic-N for the para configuration in the orientaion 1 (para 1) and the para configuration in the orientation 2 (para 2) obtained using PBE and rev-vdW-DF2.

| N position | para1 | | para2 | |
|---|---|---|---|---|
| | $E_{\mathrm{int}}$ (meV) | $d_0$ (Å) | $E_{\mathrm{int}}$ (meV) | $d_0$ (Å) |
| | | PBE | | |
| N1 | −14 | 3.709 | −35 | 3.496 |
| N2 | −17 | 3.635 | −47 | 3.400 |
| N3 | −22 | 3.592 | −35 | 3.432 |
| N4 | −14 | 3.709 | −25 | 3.651 |
| | | rev-vdW-DF2 | | |
| N1 | −93 | 3.208 | −119 | 3.182 |
| N2 | −99 | 3.176 | −143 | 3.086 |
| N3 | −105 | 3.160 | −126 | 3.118 |
| N4 | −92 | 3.214 | −105 | 3.208 |

TABLE SXIII. Equilibrium interaction energies ($E_{\rm int}$) and distance ($d_0$) of water on graphene doped with graphitic-N for the 0-leg configuration with on-top positions obtained using PBE and rev-vdW-DF2.

| N position | 0-leg (on-top) | |
|---|---|---|
| | $E_{\rm int}$ (meV) | $d_0$ (Å) |
| | PBE | |
| N1 | −39 | 3.368 |
| N2 | −54 | 3.241 |
| N3 | −42 | 3.357 |
| N4 | −31 | 3.384 |
| | rev-vdW-DF2 | |
| N1 | −125 | 3.062 |
| N2 | −152 | 3.001 |
| N3 | −131 | 3.059 |
| N4 | −112 | 3.134 |

TABLE SXIV. Equilibrium interaction energy ($E_{\rm int}$) and distances $d_0$ for water on graphene doped with pyridinic-N [pyri-N (no H)] and pyridinic-N with H-terminated C (pyri-N) for 1-leg (orientation 2) (1-leg 2), and 2-leg (orientation 2) (2-leg 2), para configuration in the orientation 1 (para1) and para configuration in the orientation 2 (para2) obtained using PBE and rev-vdW-DF2.

| | 1-leg 2 | | 2-leg 2 | | para 1 | | para 2 | |
|---|---|---|---|---|---|---|---|---|
| | $E_{\rm int}$ (meV) | $d_0$ (Å) | $E_{\rm int}$ (meV) | $d_0$ (Å) | $E_{\rm int}$ (meV) | $d_0$ (Å) | $E_{\rm int}$ (meV) | $d_0$ (Å) |
| | | | | pyri-N (no H) | | | | |
| PBE | −86 | 3.284 | −63 | 3.323 | − 2 | 3.789 | −14 | 3.379 |
| rev-vdW-DF2 | −183 | 3.096 | −162 | 3.102 | − 77 | 3.102 | −93 | 3.086 |
| | | | | pyri-N | | | | |
| PBE | −42 | 3.493 | −44 | 3.448 | −11 | 3.406 | −23 | 3.465 |
| rev-vdW-DF2 | −134 | 3.075 | −150 | 3.091 | −104 | 2.920 | −113 | 3.011 |

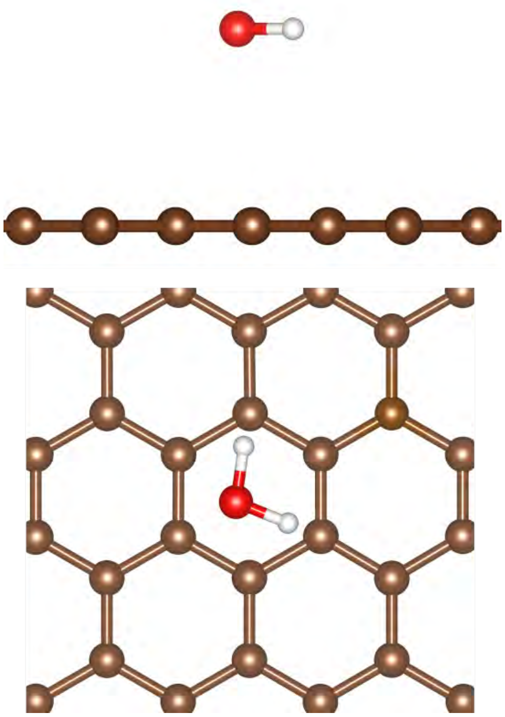

FIG. S1. Side (upper panel) and top (lower panel) views of the water adsorption configuration on pristine graphene for the parallel configuration (para). H, C, N, and O atoms are represented by white, brown, silver and red spheres, respectively

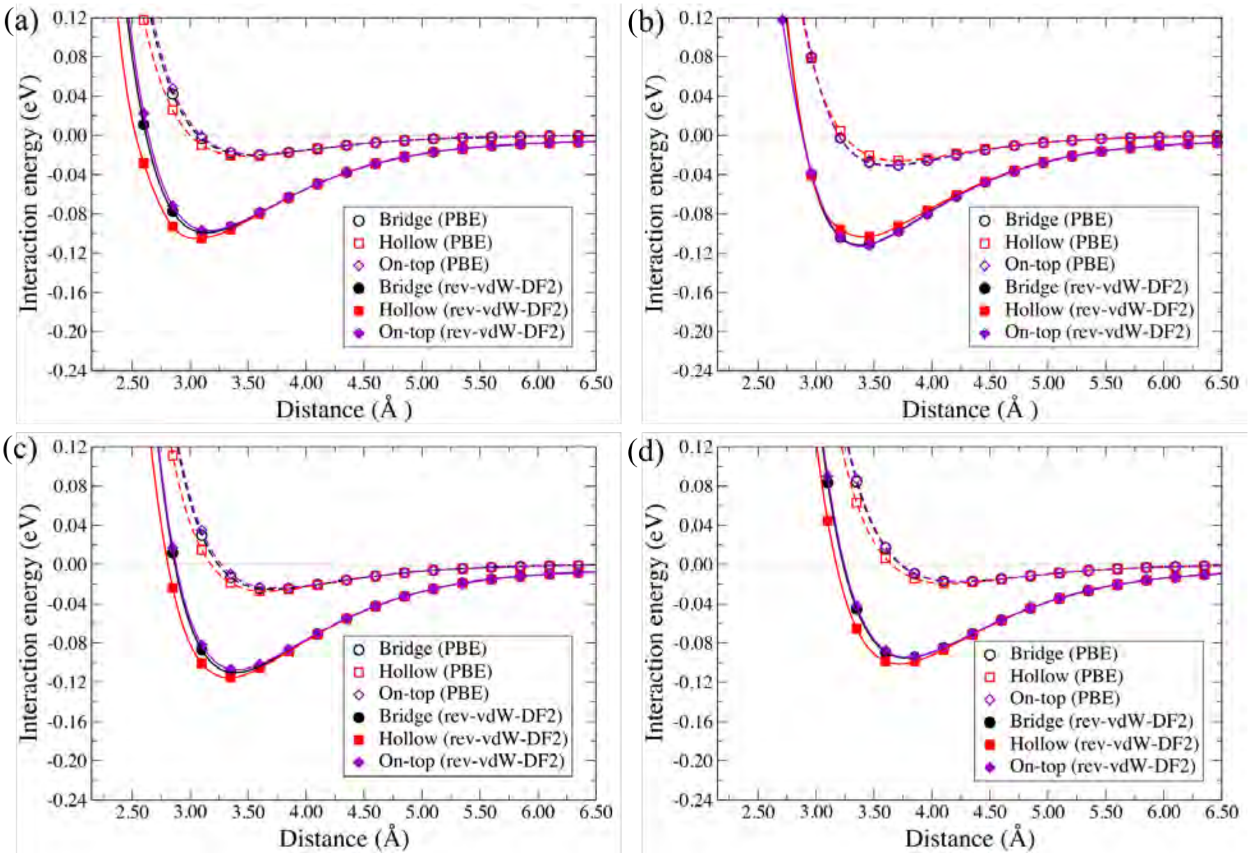


FIG. S2. Interaction energy of water with pristine graphene as a function water-surface distance for (a) 0-leg, (b) 1-leg, (c) 2-leg, and (d) para configurations on different adsorption sites.

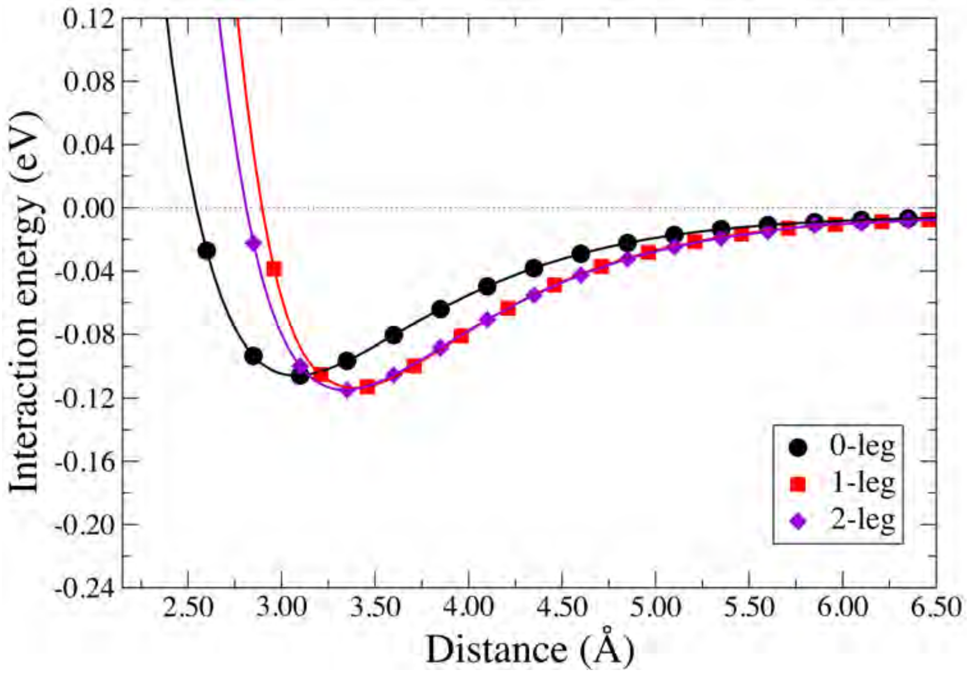


FIG. S3. Interaction energy of water with pristine graphene as a function water-graphene distance, obtained using rev-vdW-DF2. The lattice constant of graphene was optimized using rev-vdW-DF2.

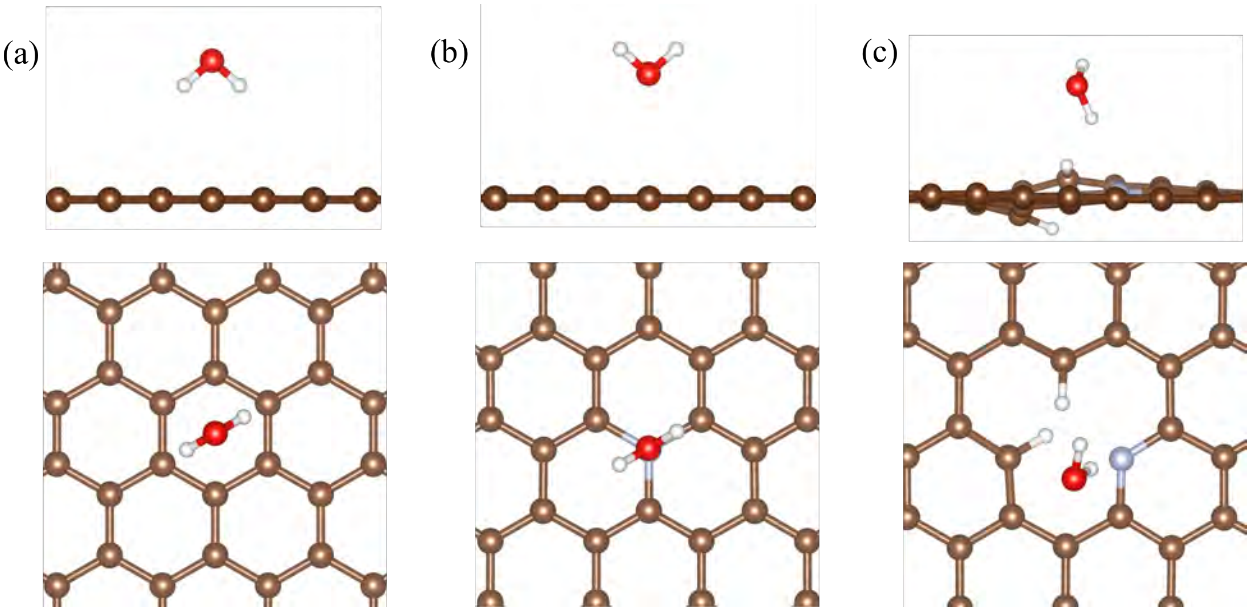


FIG. S4. Fully optimized structures for most stable water adsorption configurations on (a) prisitine graphene, (b) graphene doped with graphitic-N without H termination, and (c) graphene doped with pyridinic-N with H termination (2-leg, 0-leg and 1-leg configurations, respectively).

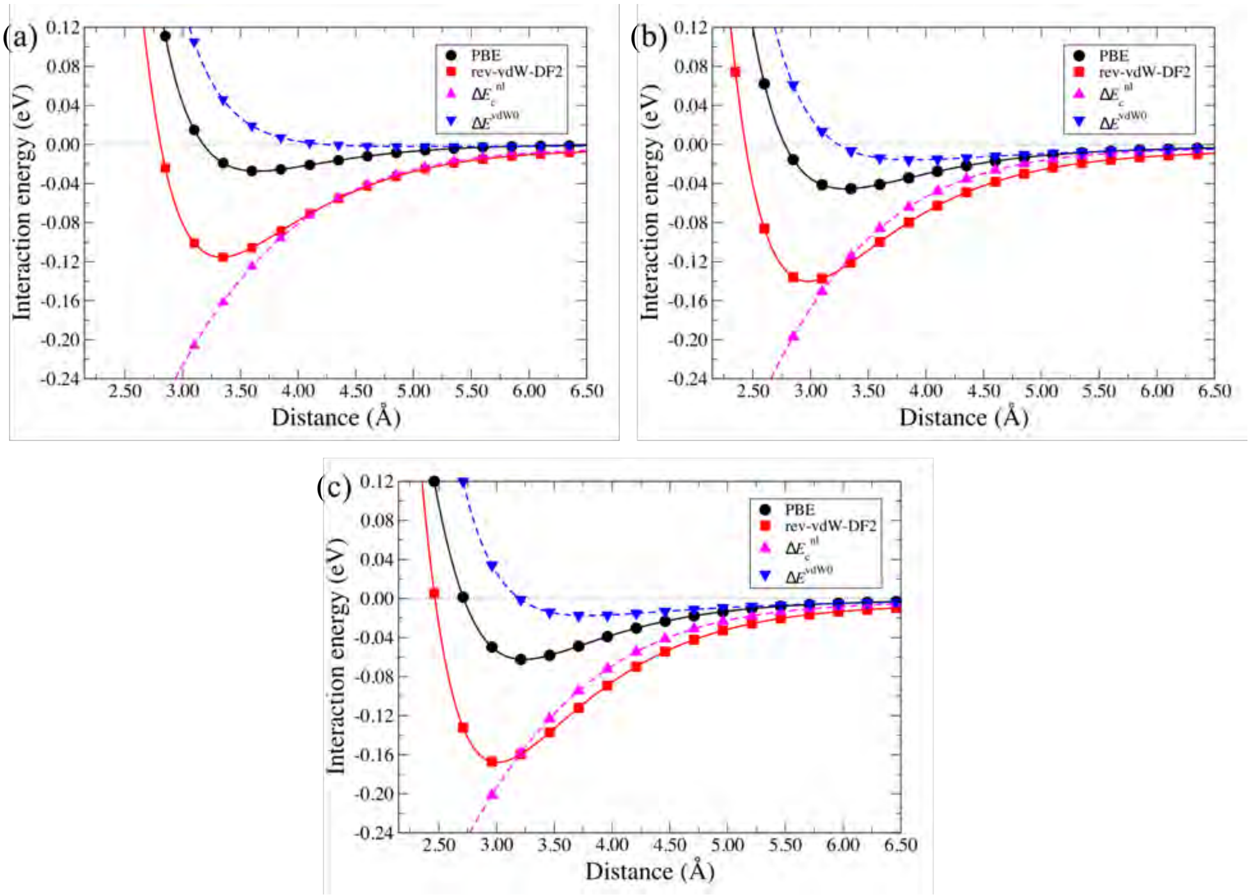


FIG. S5. Interaction energy of water for the 2-leg, 0-leg and 1-leg configurations on (a) pristine graphene, (b) graphitic-N doped and (c) pyridinic-N doped with H-terminated graphene, as a function water-surface distance, obtained using PBE and rev-vdW-DF2 functionals, respectively. For the latter, the contributions from the nonlocal correlation ($\Delta E_c^{\mathrm{nl}}$) and the rest ($\Delta E^{\mathrm{vdW0}}$) are shown.

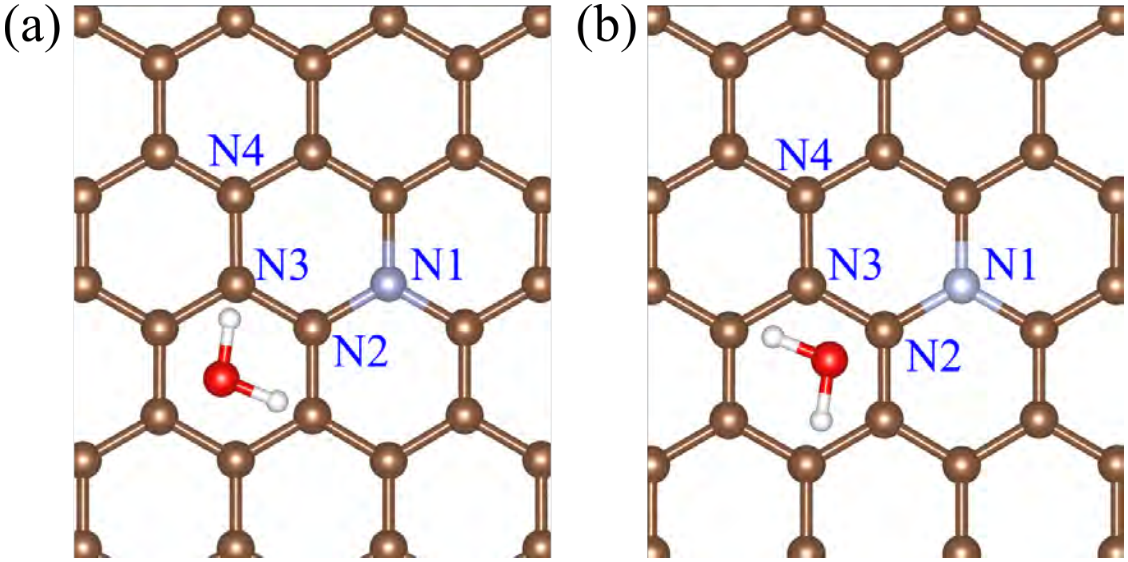


FIG. S6. Adsorption geometries of the water molecule on graphene doped with graphitic N for (a) para configuration in the orientation 1 (para 1) and (b) para configuration in the orientation 2 (para 2).

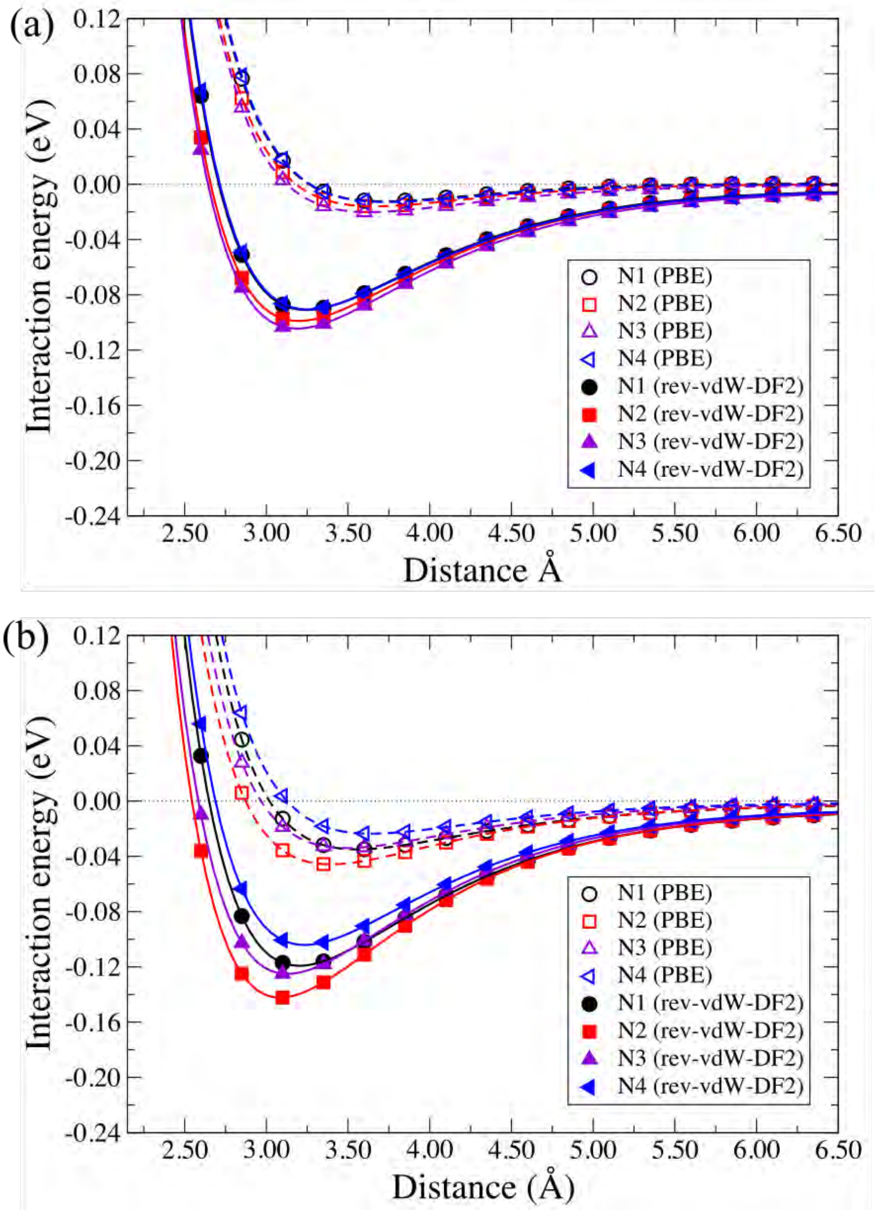


FIG. S7. Interaction energy of water with graphene doped with graphitic-N as a function of water-graphene distance for (a) para configuration in the orientation 1 (para 1) and (b) para configuration in the orientation 2 (para 2).

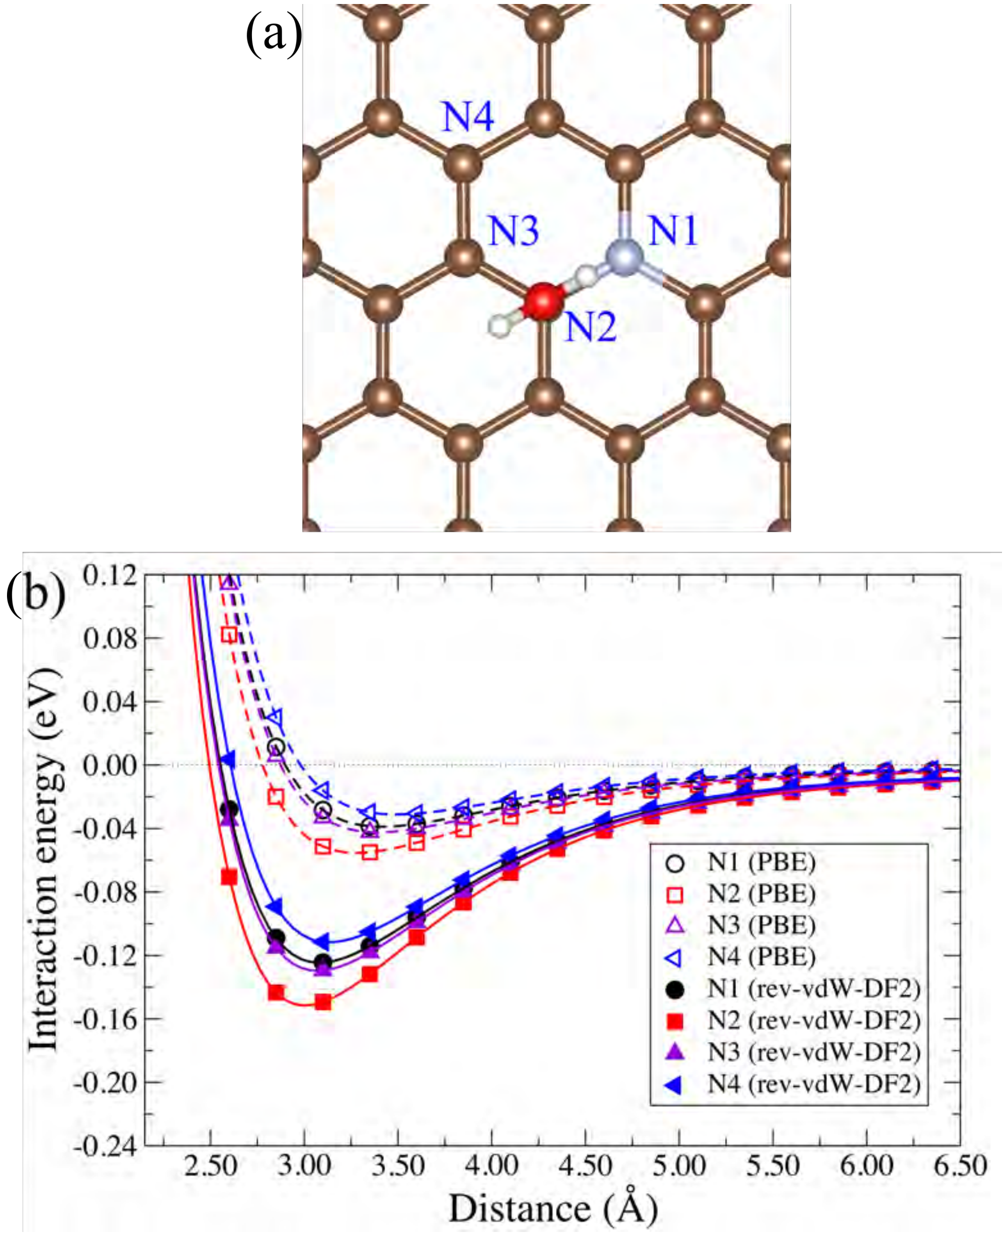


FIG. S8. (a) Adsorption geometry and (b) interaction energy as a function water-graphene distance for the 0-leg water configuration on the top-site of graphene doped with graphitic-N.

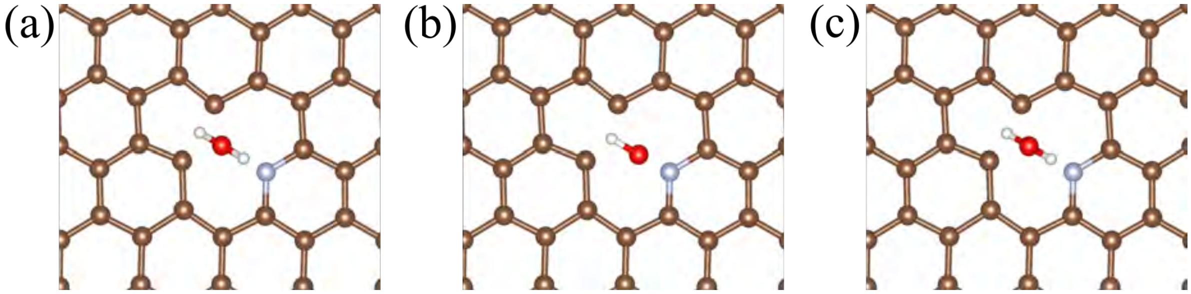

FIG. S9. Water adsorption configurations on graphene doped with pyridinic-N and non-H-terminated C for (a) 0-leg configuration, (b) 1-leg configuration (orientation 1) (1-leg 1), and (c), 2-leg (orientation 1) (2-leg 1) configuration.

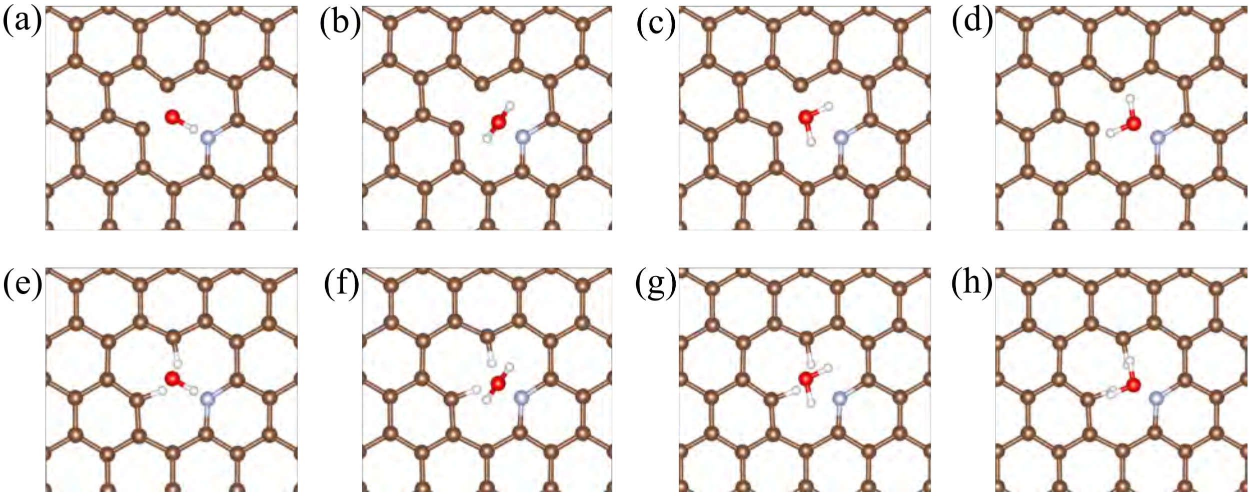

FIG. S10. Water adsorption configurations on graphene doped with pyridinic-N and non-H-terminated C for (a) 1-leg configuration (orientation 2) (1-leg 2), (b) 2-leg configuration (orientation 2) (2-leg 2), (c) para configuration in the orientation 1 (para 1), and (d) para configuration in the orientation 2 (para 2), and those on graphene doped with pyridinic-N and H-terminated C for (e) 1-leg 2, (f) 2-leg 2, (g) para 1, and (h) para 2 configurations.

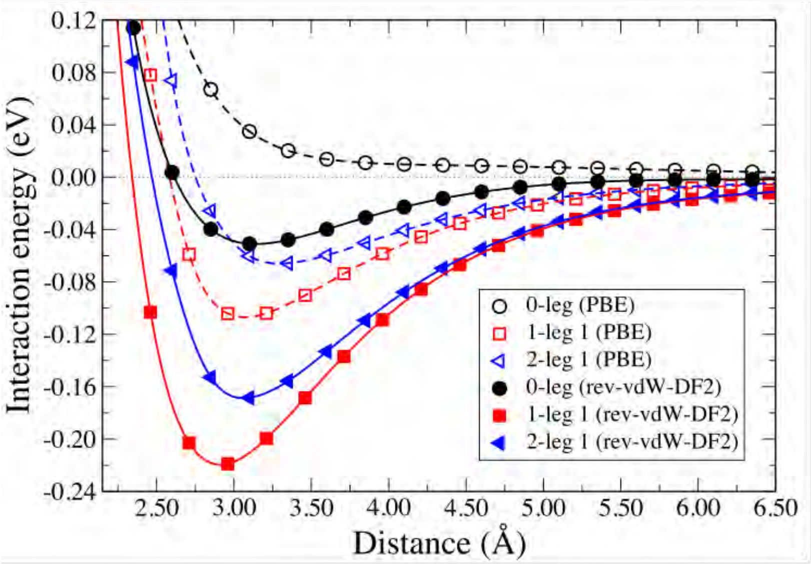


FIG. S11. Interaction energy of water with graphene doped with pyridinic-N and non-H-terminated C, as a function of water-surface distance for 0-leg, 1-leg, and 2-leg configurations. For the 1-leg and 2-leg configuration, the orientation 1 (1-leg 1) was employed.

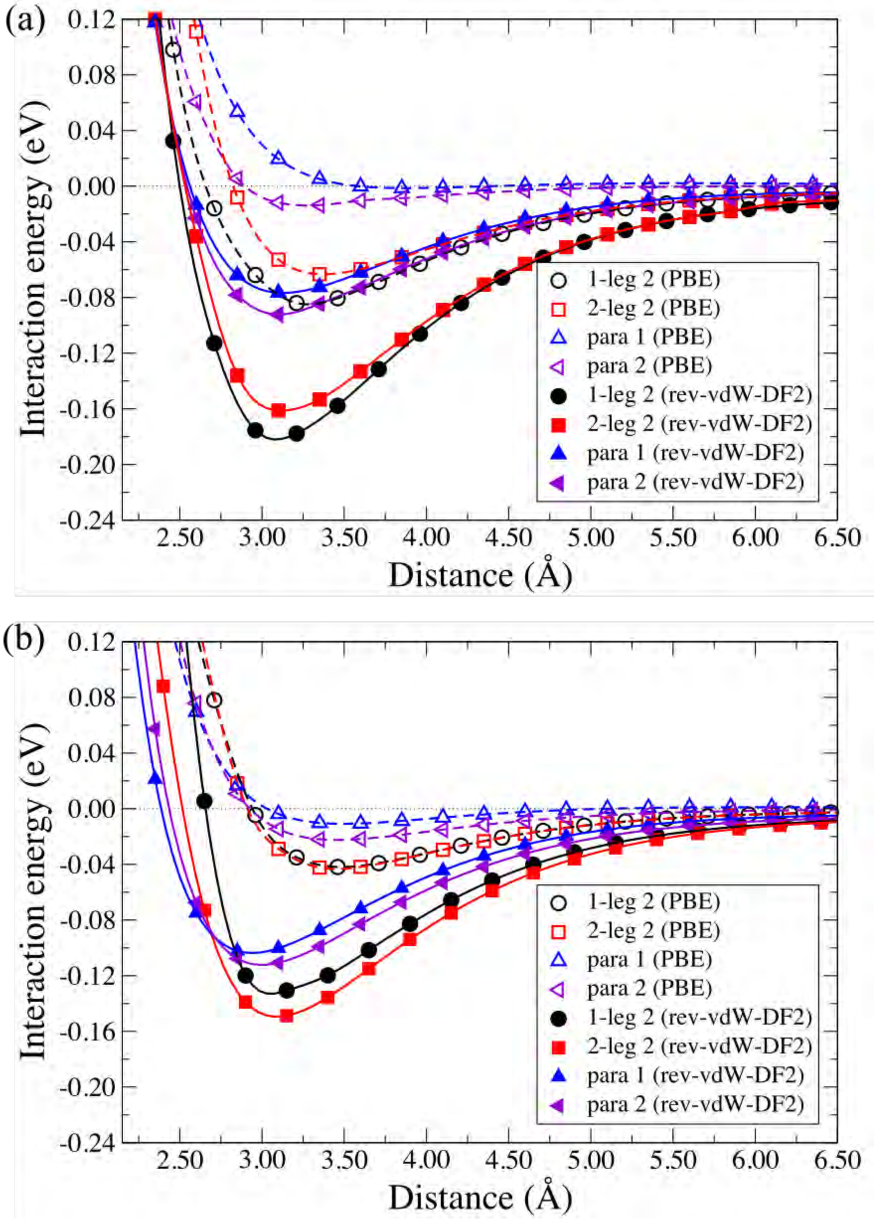


FIG. S12. Interaction energy of water with graphene doped with (a) pyridinic-N with non-H-terminated C and (b) pyridinic-N, as a function of water-graphene distance for 0-leg, 1-leg, and 2-leg configurations. For the 1-leg and 2-leg configurations, the orientation 2 (1-leg 2) was employed.

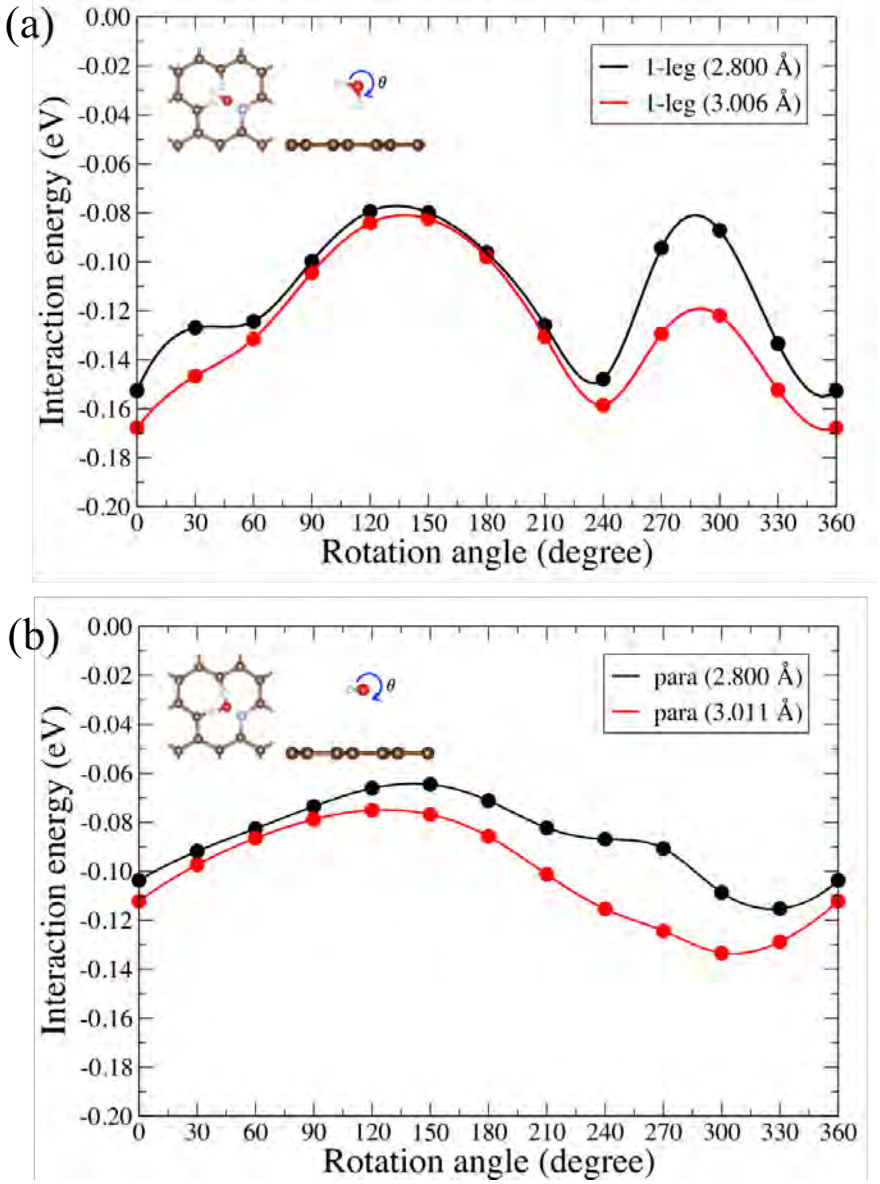


FIG. S13. Interaction energy of water adsorbed on graphene doped with pyridinic-N as a function of rotation angle around O of water for (a) 1-leg and (b) para configurations. The rotation angle is measured with respect to the equilibrium one at the heights of 3.006 Å and 3.011 Å for 1-leg and para configurations, respectively. Different water heights are considered.

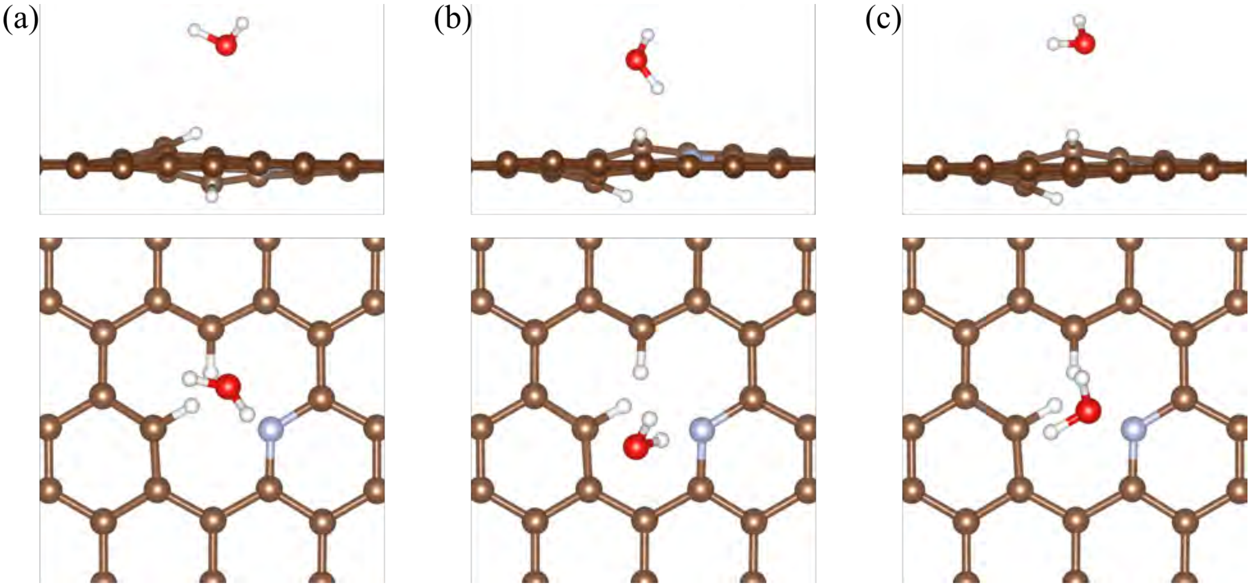


FIG. S14. Fully optimized structures for water molecules in (a) 0-leg, (b) 2-leg, and (c) para configurations on graphene doped with pyridinic-N.

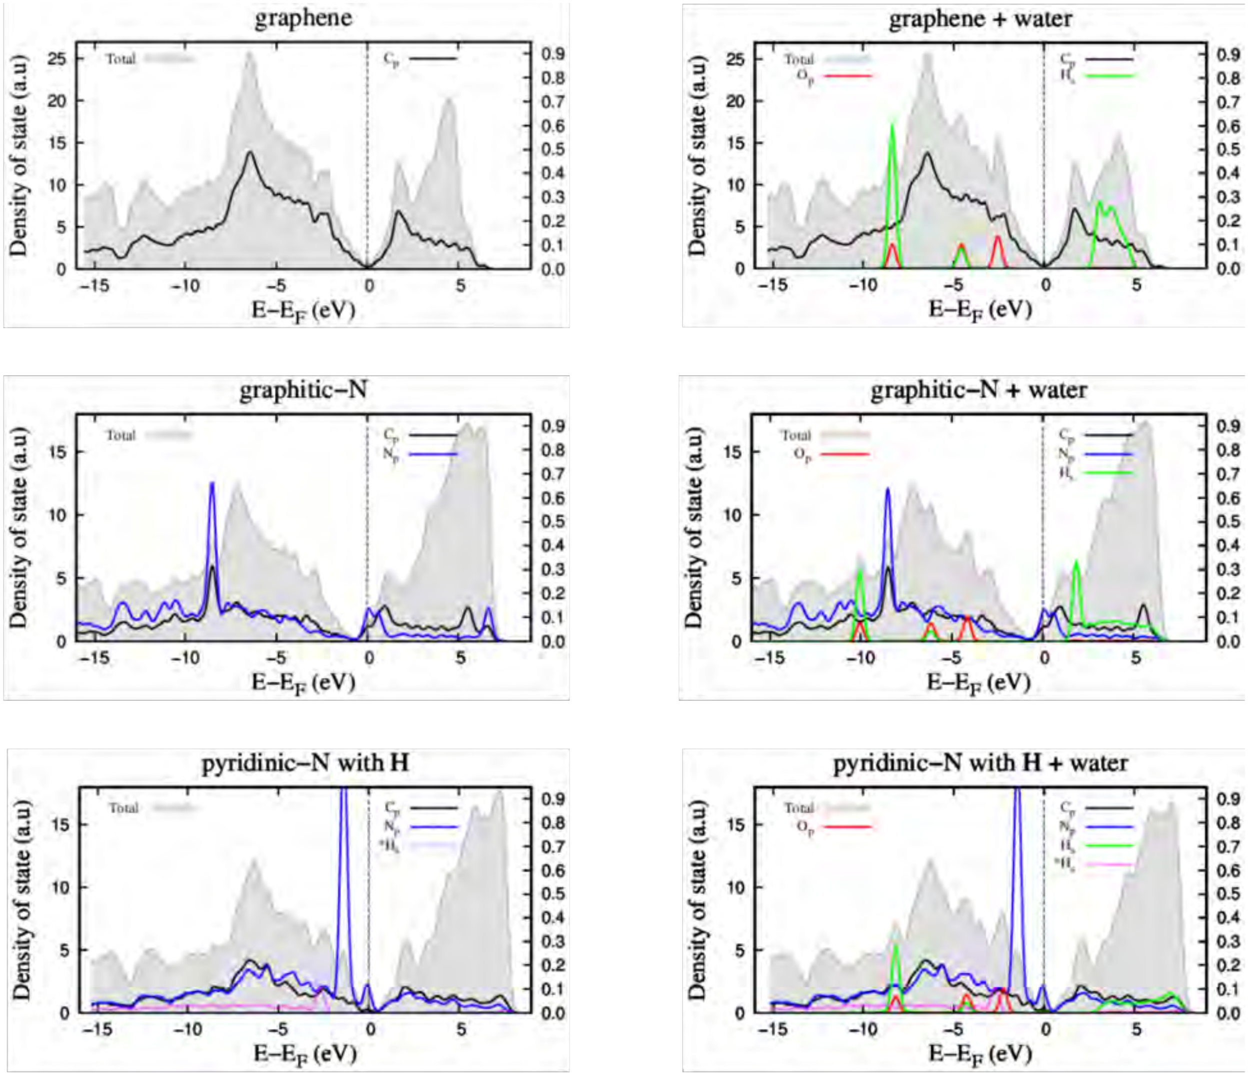


FIG. S15. Total and partial density of state for C, N and H atoms in the graphene structure nearest to the water molecules on three difference surfaces. Those in the absence of water (left panels) and those with water in the most stable configuration are shown. For the clarity of the graph, the plots are divided into two legends based on magnitude: Left (right) legend corresponds to the total (partial) density of states.

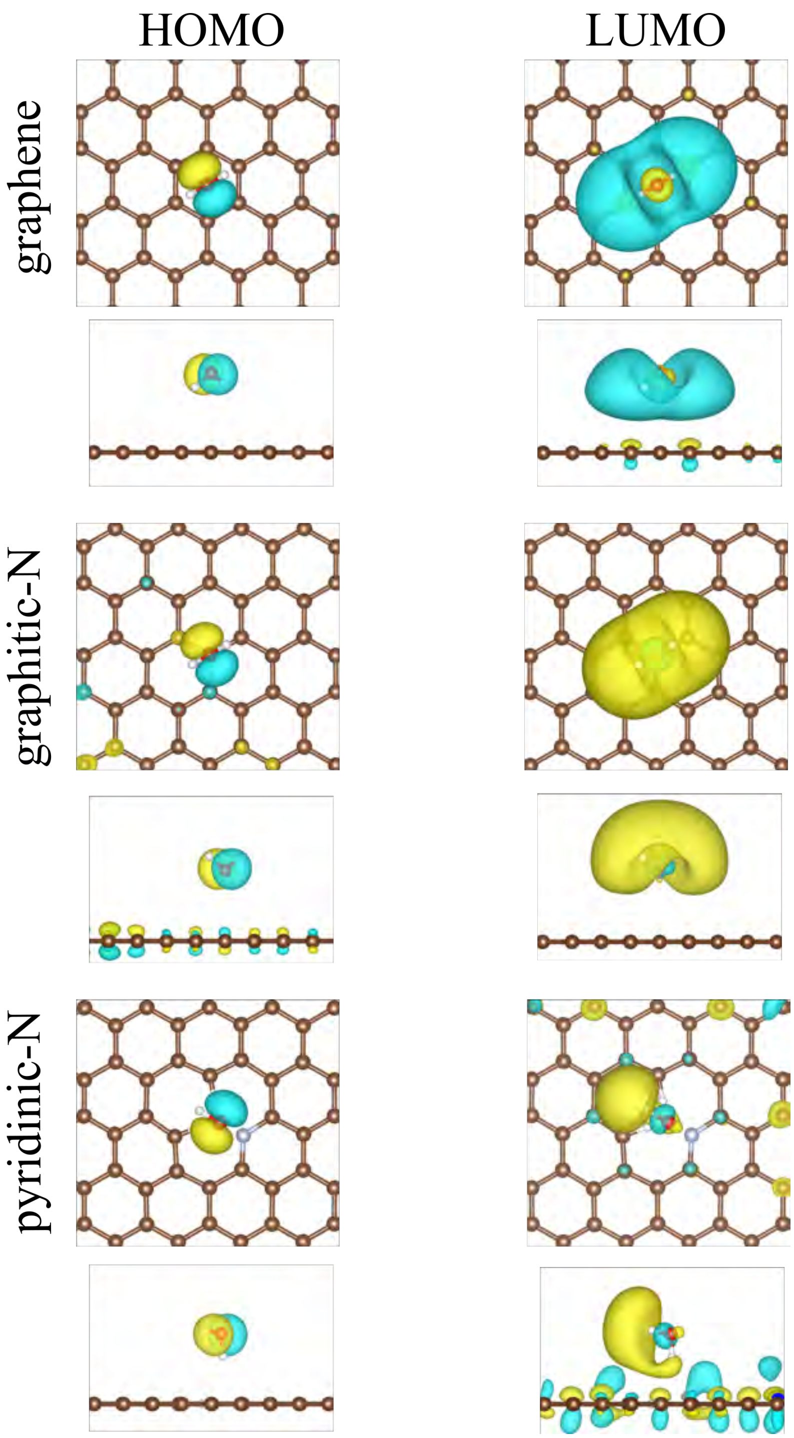


FIG. S16. Wave functions corresponding to the highest occupied molecular orbital (HOMO) and lowest unoccupied molecular orbital (LUMO) of water for the 2-leg, 0-leg and 1-leg configurations on the (top) pristine, (middle) graphitic-N doped, and (bottom) pyridinic-N doped with H-terminated graphene.

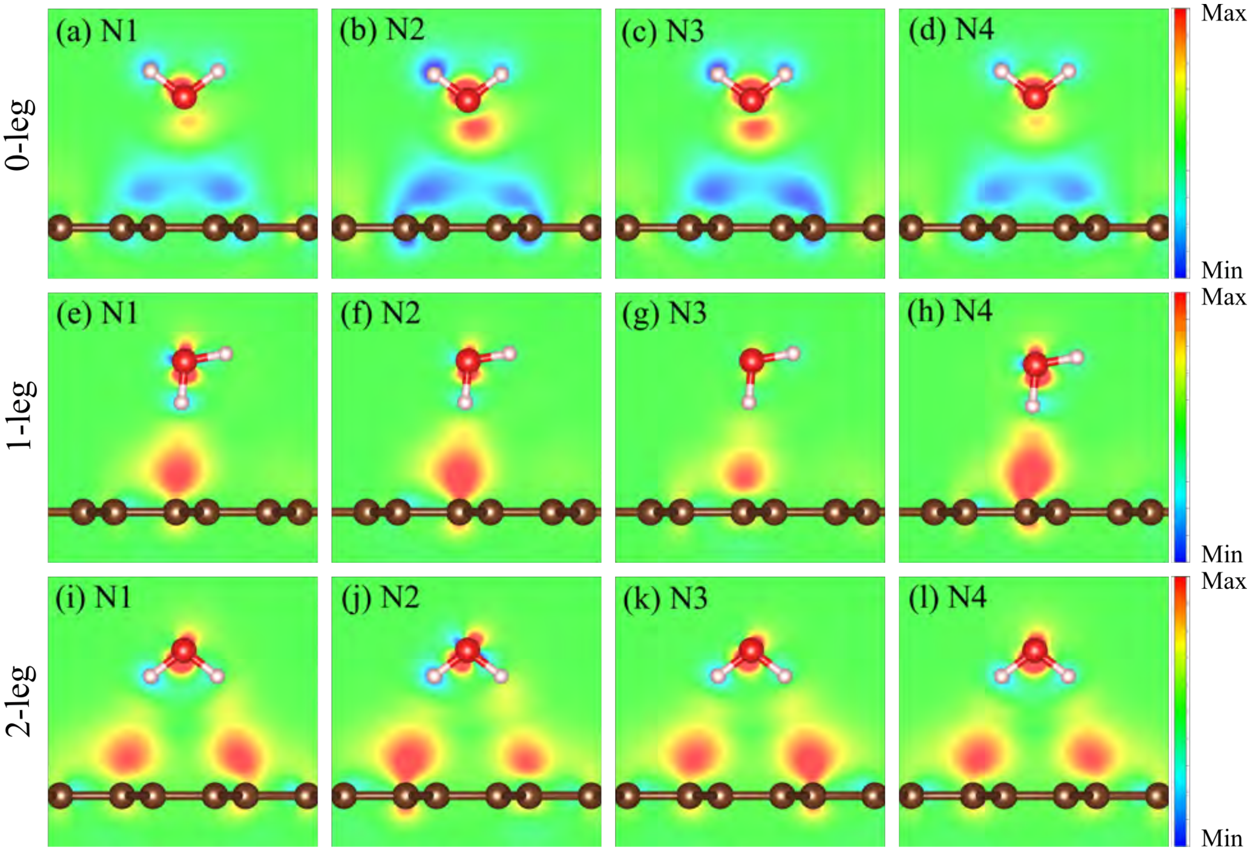


FIG. S17. Charge-density difference ($\Delta\rho$) of water on graphitic-N for 0-leg, 1-leg and 2-leg configurations with the black-red arrow indicated the N-doped positions at N1, N2, N3 and N4, respectively.The Maximum (minimum) value of $\Delta\rho$ is $1.35 \times 10^{-2}$ ($-1.35 \times 10^{-2}$) $e$ Å$^{-3}$.

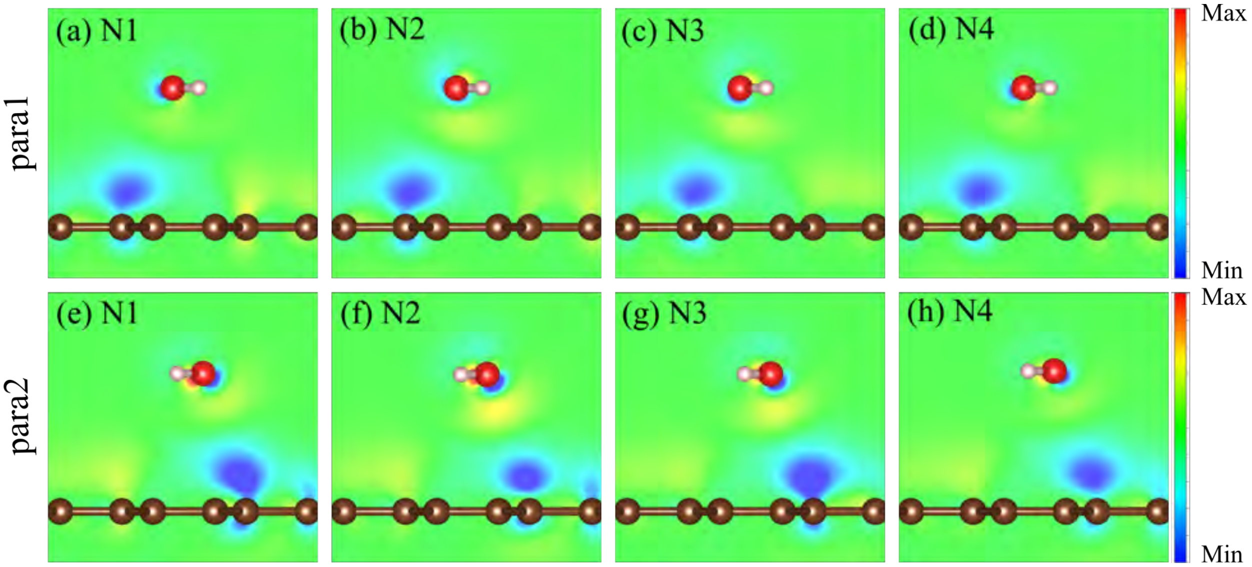


FIG. S18. Charge-density difference ($\Delta\rho$) of the water molecule on graphene doped with graphitic-N for (a)-(d) the para configuration in the orientation 1 (para1) and (e)-(f) that in the orientation 2 (para2). Different N positions (N1-N4) are considered. The Maximum (minimum) value of $\Delta\rho$ is $1.35 \times 10^{-2}$ ($-1.35 \times 10^{-2}$) $e$ Å$^{-3}$.

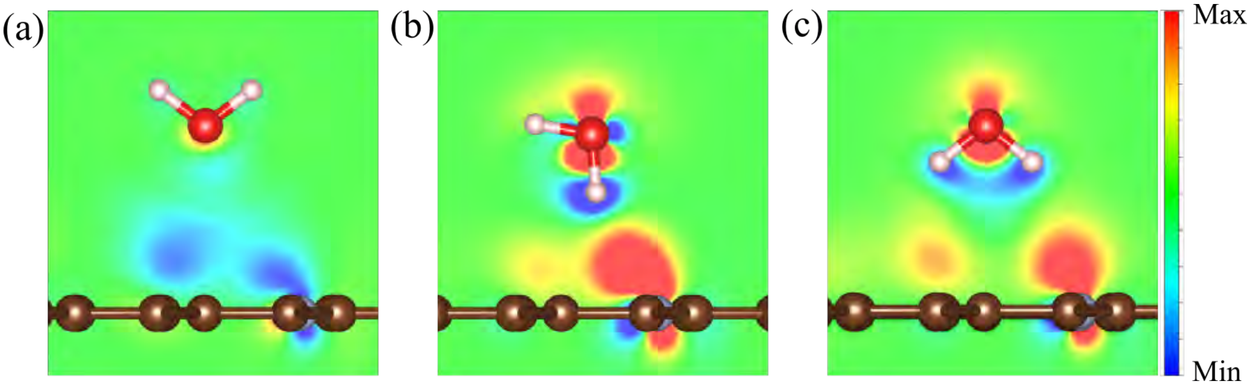


FIG. S19. Charge-density difference ($\Delta\rho$) of water molecules on graphene doped with pyridinic-N with no-H-terminated C atoms for (a) 0-leg , (b) 1-leg 1, (c) 2-leg 1 configurations. The Maximum (minimum) value of $\Delta\rho$ is $1.35 \times 10^{-2}$ ($-1.35 \times 10^{-2}$) $e$ Å$^{-3}$.

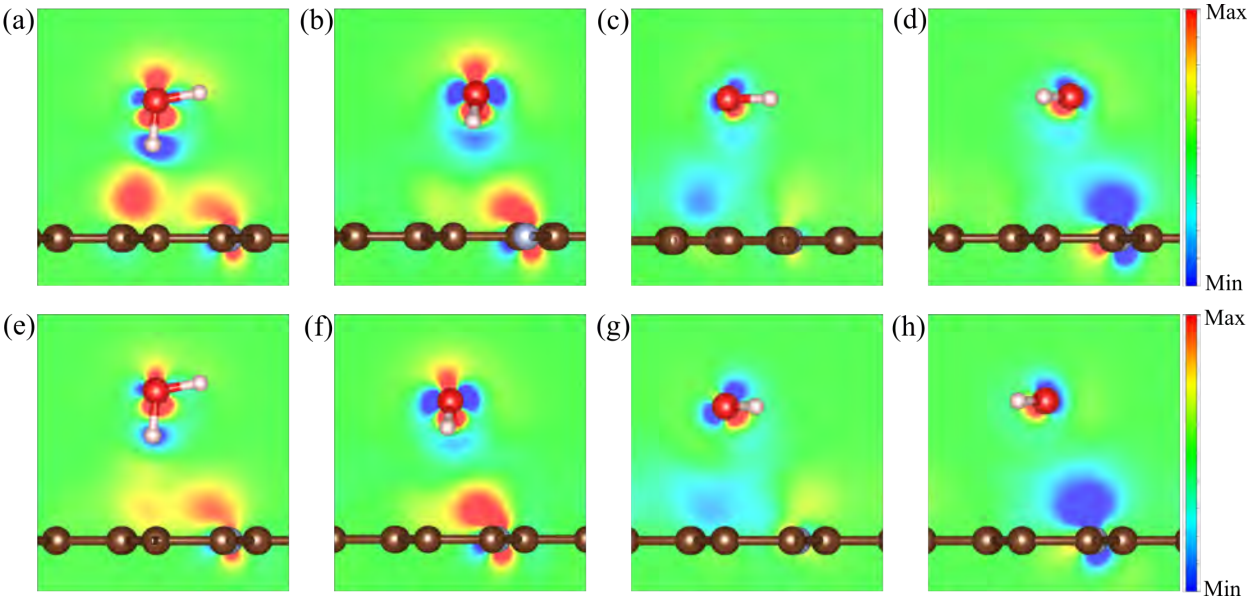


FIG. S20. Charge-density difference ($\Delta\rho$) of water molecules on graphene doped with pyridinic-N with non-H-terminated C atoms for (a) 1-leg 2 , (b) 2-leg 2, (c) para1, and (d) para 2 configurations, and those with H-terminated C atoms for (a) 1-leg 2 , (b) 2-leg 2, (c) para 1, and (d) para 2 configurations. The Maximum (minimum) value of $\Delta\rho$ is $1.35 \times 10^{-2}$ ($-1.35 \times 10^{-2}$) $e$ Å$^{-3}$.

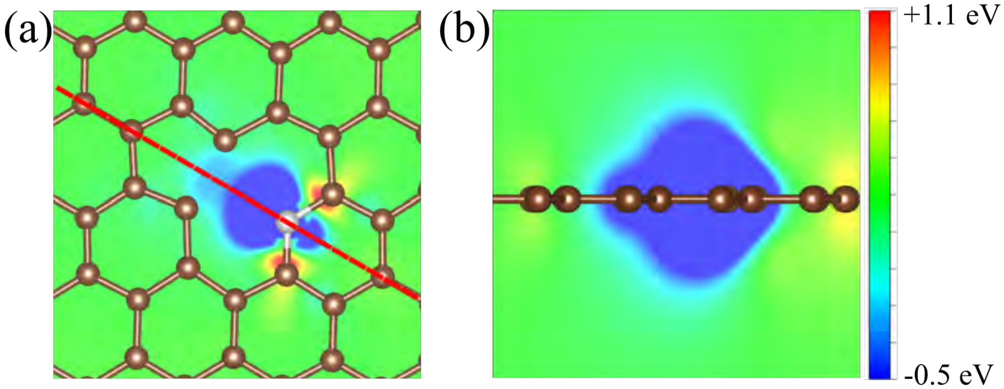


FIG. S21. (a) top and (b) side views of the Hatree potential difference for pyridinic-N without H termination of C. The red dotted line indicates the lattice plane shown in (b).

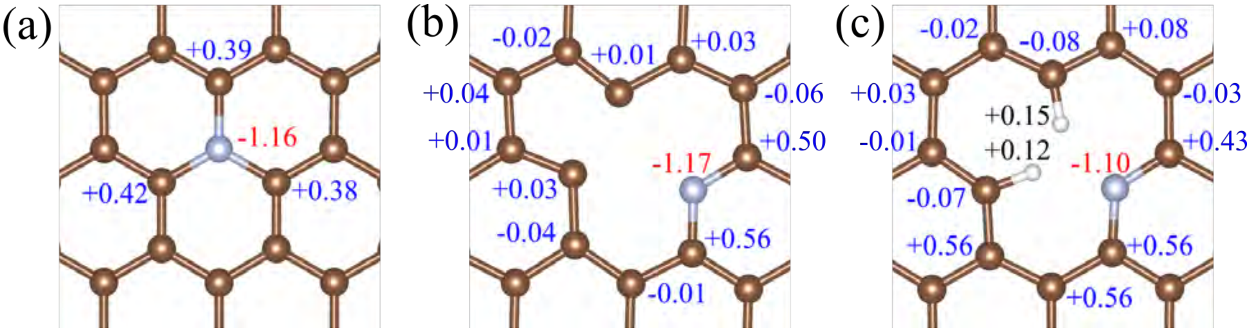


FIG. S22. Bader charge analysis for (a) graphitic-N, (b) pyridinic-N with non-H-terminated C atoms, and (c) pyridinic-N with H-terminated C atoms structures. The calculated net charges for C, N and H atoms are shown in blue, red and black, respectively.

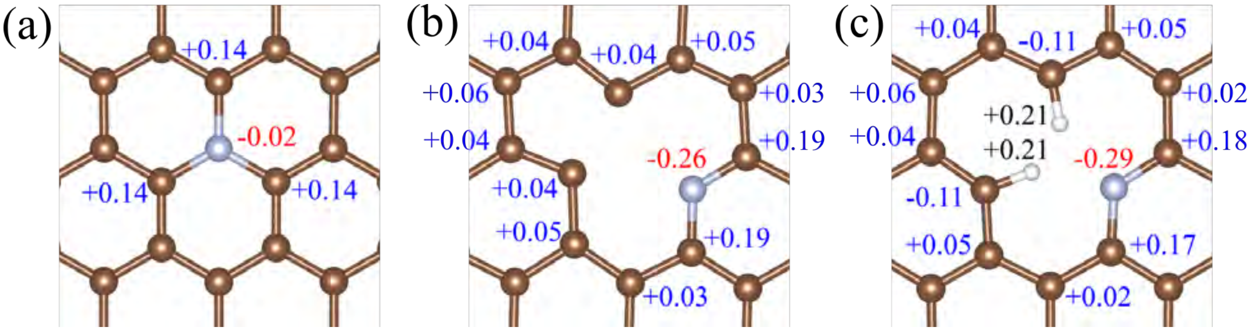


FIG. S23. Löwdin's charge population analysis for (a) graphitic-N, (b) pyridinic-N with non-H-terminated C atoms, and (c) pyridinic-N with H-terminated C atoms structures. The calculated net charges for C, N and H atoms are shown in blue, red and black, respectively.

[1] J. G. Brandenburg, A. Zen, D. Alfè, and A. Michaelides, Interaction between water and carbon nanostructures: How good are current density functional approximations?, J. Chem. Phys. **151**, 164702 (2019).

[2] T. Kurita, S. Okada, and A. Oshiyama, Energetics of ice nanotubes and their encapsulation in carbon nanotubes from density-functional theory, Phys. Rev. B **75**, 205424 (2007).

[3] O. Leenaerts, B. Partoens, and F. M. Peeters, Adsorption of $H_2O$, $NH_3$, CO, $NO_2$, and NO on graphene: A first-principles study, Phys. Rev. B **77**, 125416 (2008).
